# Supplementary material for: Energy-energy correlators within $Z$-tagged jets in proton-proton collisions at $\sqrt{s}$ = 13 TeV
Source: arXiv:2610.14221 source file (2026-10-09)
Supplement: Supplementary file 2 [file appendix.tex]

% ===============================================================================
% Purpose: appendix to the standard template: standard symbol alises from Ulrik
% Author: Tomasz Skwarnicki
% Created on: 2009-09-24
% ===============================================================================

%{\noindent\normalfont\bfseries\Large Appendices}
\section*{Appendices}

\appendix

\section{Standard References}
\label{sec:StandardReferences}
Below is a list of common references, as
well as a list of all \lhcb publications.
As they are already in prepared bib files, they can be used as simply as
\texttt{\textbackslash cite\{LHCb-DP-2008-001\}} to get the \lhcb detector paper.
The references are defined in the files \texttt{main.bib},  \texttt{LHCb-PAPER.bib},
\texttt{LHCb-CONF.bib}, \texttt{LHCb-DP.bib} \texttt{LHCb-TDR.bib} files, with obvious contents.
Each of these have their \texttt{LHCb-ZZZ-20XX-0YY} number as their cite code.
If you believe there is a problem with the formatting or
content of one of the entries, then get in contact with the Editorial
Board rather than just editing it in your local file,
since you are likely to need the latest version just before submitting the article.

%%%%%%%%%%%%%%%%%%%%%%%%%%%%%%%%%%
\newcommand{\showcite}[1]{\texttt{#1}~\cite{#1}}%
\newcommand{\revshowcite}[1]{\begin{minipage}{1.2cm}\cite{#1}\end{minipage}\texttt{#1}}%
%%%%%%%%%%%%%%%%%%%%%%%%%%%%%%%%%%
\begin{center}
  \begin{longtable}{ll}
\caption{\small Standard references.}\label{tab:Refs}
\endfirsthead
\multicolumn{2}{c}{ -- continued from previous page.}
\endhead
\endfoot
\endlastfoot
\hline
Description & \begin{minipage}{1cm}Ref.\end{minipage}\texttt{cite} code \\
\hline % standard physics papers
Lee, Weinberg, Zumino & \revshowcite{Lee:1967iu}  \\ % {Weinberg:1967} \\
Cabibbo, Kobayashi, Maskawa & \revshowcite{Cabibbo:1963yz,*Kobayashi:1973fv}  \\ % {Cabibbo:1963yz,*Kobayashi:1973fv} \\
Quark Model & \revshowcite{GellMann:1964nj,*Petermann:1965qlk,*Zweig:352337}  \\ % {GellMann:1964nj,*Zweig:352337} \\
Baryon asymmetry \& SM \CP &  \revshowcite{Gavela:1994dt}  \\ % {Gavela:1994dt} \\
Baryon asymmetry \& SM \CP &  \revshowcite{Gavela:1993ts}  \\ % {Gavela:1993ts} \\
EW Baryogenesis \& \CP &  \revshowcite{Huet:1994jb}  \\ % {Huet:1994jb} \\
Dalitz Plot\footnote{Dalitz invented the method, Fabri added relativistic corrections.} & \revshowcite{Dalitz:1953cp,*Fabri:1954zz} \\
\hline % physics resources
PDG 2024  & \revshowcite{PDG2024} \\
PDG 2022  & \revshowcite{PDG2022} \\
PDG 2020  & \revshowcite{PDG2020} \\
%PDG 2019  & \revshowcite{PDG2019} \\
%PDG 2018 & \revshowcite{PDG2018} \\
%PDG 2016 & \revshowcite{PDG2016}  \\ % {PDG2016} \\
%PDG 2014 & \revshowcite{PDG2014}  \\ % {PDG2014} \\
HFLAV Zenodo record\footnote{See Sec.~\ref{sec:References} for usage.} & \revshowcite{HFLAV23-Zenodo-XXXXXX} \\
\sout{HFLAV 2023}\footnote{Use the Zenodo record instead.} & \revshowcite{HFLAV23}  \\ 
HFLAV 2021 & \revshowcite{HFLAV21}  \\ 
HFLAV 2018 & \revshowcite{HFLAV18}  \\ 
%HFLAV 2016 & \revshowcite{HFLAV16}  \\ 
%HFLAV (pre-2016)  & \revshowcite{Amhis:2014hma}  \\ 
CKMfitter group & \revshowcite{CKMfitter2005}  \\ % {CKMfitter2005} \\
CKMfitter group & \revshowcite{CKMfitter2015}  \\ % {CKMfitter2015} \\
UTfit (Standard Model/CKM) & \revshowcite{UTfit-UT}  \\ % {UTfit-UT} \\
UTfit (New Physics) & \revshowcite{UTfit-NP}  \\ % {UTfit-NP} \\
\hline % computing
\pythia8.3 & \revshowcite{10.21468/SciPostPhysCodeb.8,*10.21468/SciPostPhysCodeb.8-r8.3}  \\ 
\pythia8.2 & \revshowcite{Sjostrand:2014zea}  \\ 
\pythia8.1 & \revshowcite{Sjostrand:2007gs,*Sjostrand:2006za}  \\ 
\pythia6    & ~~~~~~use only  \verb=Sjostrand:2006za= \\ 
\lhcb \pythia tuning & \revshowcite{LHCb-PROC-2010-056}  \\ % {LHCb-PROC-2010-056} \\
\evtgen & \revshowcite{Lange:2001uf}   \\ % {Lange:2001uf} \\
%\photos & \revshowcite{Golonka:2005pn}   \\ % {Golonka:2005pn} \\
\photos & \revshowcite{davidson2015photos}   \\ % {davidson2015photos} \\
\geant & \revshowcite{Allison:2006ve, *Agostinelli:2002hh}  \\ % {Allison:2006ve, *Agostinelli:2002hh} \\
\lhcb simulation & \revshowcite{LHCb-PROC-2011-006}  \\ % {LHCb-PROC-2011-006} \\
{\tt RapidSim} & \revshowcite{Cowan:2016tnm}  \\ % {Cowan:2016tnm} \\
\dirac & \revshowcite{Tsaregorodtsev:2010zz,*BelleDIRAC}  \\ % {Tsaregorodtsev:2010zz, *BelleDIRAC}  \\
\hline % LHCb-specific
HLT2 topological trigger & \revshowcite{BBDT}  \\ % {BBDT} \\
Topological trigger reoptimization --- Run 2 & \revshowcite{LHCb-PROC-2015-018}\\
Turbo and real-time alignment --- Run 2 & \revshowcite{LHCb-PROC-2015-011}  \\
TisTos method & \revshowcite{LHCb-DP-2012-004}  \\
%TisTos method & \revshowcite{LHCb-PUB-2014-039}  \\
Allen &  \revshowcite{Aaij:2019zbu}  \\
Networks use in HLT &  \revshowcite{Kitouni:2021fkh}  \\
Stripping & \revshowcite{Stripping} \\
Sprucing & \revshowcite{Sprucing} \\
PIDCalib  & \revshowcite{LHCb-PUB-2016-021} \\ 
PID performance (for Run~1/Run~2) & \revshowcite{LHCb-DP-2012-003}/  ???? \\
Ghost probability & \revshowcite{DeCian:2255039}  \\ % {DeCian:2255039}\\
Primary vertex reconstruction & \revshowcite{Kucharczyk:1756296} \\
DecayTreeFitter & \revshowcite{Hulsbergen:2005pu}  \\ % {Hulsbergen:2005pu} \\
SMOG & \revshowcite{FerroLuzzi:2005em,*SmogPhDThesis}
\\ % {FerroLuzzi:2005em} \\
SMOG2 & \revshowcite{Smog2} \\
Run~2 tagging & \revshowcite{Fazzini:2018dyq}\\
OS \kaon, \muon, \electron and VS tagging & \revshowcite{LHCb-PAPER-2011-027}\\
OS charm tagging & \revshowcite{LHCb-PAPER-2015-027}\\
SS kaon tagging & \revshowcite{LHCb-PAPER-2015-056}\\
SS proton and pion tagging & \revshowcite{LHCb-PAPER-2016-039}\\
Inclusive tagging & \revshowcite{LHCb-PAPER-2025-024}\\
Recommendations for multiple candidates & \revshowcite{Koppenburg:2017zsh} \\
Material in inner tracker & \revshowcite{LHCb-2008-054} \\
\multicolumn{2}{l}{See also Table~\ref{tab:LHCb-DPs} for LHCb performance references.}\\
\hline % selection
\sPlot & \revshowcite{Pivk:2004ty}  \\ % {Pivk:2004ty} \\
sFit & \revshowcite{Xie:2009rka}  \\ % {Xie:2009rka} \\
Punzi's optimization & \revshowcite{Punzi:2003bu}  \\ % {Punzi:2003bu} \\
BDT & \revshowcite{Breiman}  \\ % {Breiman} \\
BDT training & \revshowcite{AdaBoost}  \\ % {AdaBoost} \\
TMVA\footnote{Do not cite this instead of the actual reference for the  MVA being used.}  & \revshowcite{Hocker:2007ht,*TMVA4}  \\ % {Hocker:2007ht,*TMVA4} \\
k-fold &  \revshowcite{kFold} \\
RooUnfold & \revshowcite{Adye:2011gm}  \\ % {Adye:2011gm} \\
scikit-learn & \revshowcite{Scikit-learn-paper}  \\ % {Scikit-learn-paper} \\
pyhf:2021 & \revshowcite{py:pyhf:2021} \\
uproot & \revshowcite{py:uproot} \\
hist & \revshowcite{py:hist} \\
particle & \revshowcite{py:particle} \\
mplhep & \revshowcite{py:mplhep} \\
scikit-hep:2020 & \revshowcite{py:scikit-hep:2020} \\
boost-histogram & \revshowcite{py:boost-histogram} \\
hepstats & \revshowcite{py:hepstats} \\
iminuit & \revshowcite{py:iminuit} \\
hepunits & \revshowcite{py:hepunits} \\
vector & \revshowcite{py:vector} \\
awkward-array & \revshowcite{py:awkward-array} \\
zfit:2020 & \revshowcite{py:zfit:2020} \\
zfit & \revshowcite{py:zfit} \\
phasespace:2019 & \revshowcite{py:phasespace:2019} \\
pytorch & \revshowcite{py:pytorch} \\
\textsc{Laura}$^{++}$ & \revshowcite{Back:2017zqt}  \\ % {Back:2017zqt} \\
\texttt{hep\_ml} & \revshowcite{Rogozhnikov:2016bdp}  \\ % {Rogozhnikov:2016bdp} \\
\texttt{root\_numpy} & \revshowcite{root-numpy}  \\
\texttt{GammaCombo}\footnote{Always cite this along with Ref.~\cite{LHCb-PAPER-2016-032} (or Ref.~\cite{LHCb-PAPER-2021-033} if referring to the determination of $\gamma$ with charm mixing results) as {\tt\textbackslash{}cite\{GammaCombo,*LHCb-PAPER-2016-032 (*LHCb-PAPER-2021-033)\}} (unless {\tt LHCb-PAPER-2016-032} ({\tt LHCb-PAPER-2021-033}) is cited elsewhere).} & \revshowcite{GammaCombo}  \\
\tensorflow & \revshowcite{tensorflow2015-whitepaper}  \\ % {tensorflow2015-whitepaper} \\
FunTuple & \revshowcite{FunTuple} \\
\hline % Fits
Crystal Ball function\footnote{A valid alternative for most papers where the normalisation is not critical is to use the expression``Gaussian function with a low-mass power-law tail'' or ``Gaussian function with power-law tails''. In that case, no citation is needed} & \revshowcite{Skwarnicki:1986xj}  \\ % {Skwarnicki:1986xj} \\
Hypatia function & \revshowcite{Santos:2013gra}  \\ % {Santos:2013gra}\\
Modified Novosibirsk function & \revshowcite{Ikeda:1999aq} \\
Bukin function & \revshowcite{Bukin:2007} \\
Wilks' theorem & \revshowcite{Wilks:1938dza} \revshowcite{Cowan:2010js}  \\ % {Wilks:1938dza}\\
CL$_s$ method & \revshowcite{CLs}  \\ % {CLs} \\
BLUE method & \revshowcite{Nisius:2020jmf}  \\ 
Bootstrapping & \revshowcite{efron:1979}  \\ % {efron:1979} \\
Blatt--Weisskopf barrier & \revshowcite{Blatt:1952ije}  \\ % {Blatt:1952ije} \\
\hline % LHC
%%$f_s/f_d$ at 7--8\tev & \revshowcite{fsfd}  \\ % {fsfd} \\
$f_s/f_d$ at 7--8 and 13\tev & \revshowcite{LHCb-PAPER-2020-046}  \\  % updated
LHC beam energy uncertainty  & \revshowcite{PhysRevAccelBeams.20.081003}  \\ % {PhysRevAccelBeams.20.081003}\\
Exotic hadron naming conventrion & \revshowcite{LHCb-PUB-2022-013} \\
Measurement of the instrumental asymmetry &  \revshowcite{LHCb-PUB-2018-004} \\
for $\Km\pip$-pairs at LHCb in Run 2 &  \\
\hline
\end{longtable}
%  \end{tabular}
\end{center}

\begin{center}
\begin{longtable}{ll}
\caption{\small LHCb detector performance papers.}\label{tab:LHCb-DPs}
\endfirsthead
\multicolumn{2}{c}{ -- continued from previous page.}
\endhead
\endfoot
\endlastfoot
\hline
    \hline
    \texttt{LHCb-DP} number & Title \\
    \hline
    \showcite{LHCb-DP-2025-007} &  {\small Performance of the LHCb muon detector in Run 3} \\
    \showcite{LHCb-DP-2025-006} &  {\small A method for luminosity determination based on real-time hit \dots} \\
    \showcite{LHCb-DP-2025-005} &  {\small Metal Foil Detectors assembly for the beam \dots} \\
    \showcite{LHCb-DP-2025-004} &  {\small Deuteron identification via time of flight with LHCb} \\
    \showcite{LHCb-DP-2024-003} &  {\small Luminosity measurement with the LHCb RICH detectors in Run 3} \\
    \showcite{LHCb-DP-2024-002} &  {\small High-density gas target at the LHCb experiment} \\
    \showcite{LHCb-DP-2024-001} &  {\small The LHCb VELO Upgrade module construction} \\
    \showcite{LHCb-DP-2023-004} &  {\small Tracking of charged particles with nanosecond lifetimes at LHCb} \\
    \showcite{LHCb-DP-2023-003} &  {\small Momentum scale calibration of the LHCb spectrometer} \\
    \showcite{LHCb-DP-2023-002} &  {\small Helium identification with LHCb} \\
    \showcite{LHCb-DP-2023-001} &  {\small Curvature-bias corrections using a pseudomass method} \\
    \showcite{LHCb-DP-2022-002} &  {\small The LHCb Upgrade I}\\
    \showcite{LHCb-DP-2022-001} &  {\small Long-lived particle reconstruction downstream of the LHCb magnet}\\
    \showcite{LHCb-DP-2021-006} &  {\small Identification of charm jets at LHCb}\\
    \showcite{LHCb-DP-2021-004} &  {\small Performance of the LHCb RICH detectors during Run 2}\\
    \showcite{LHCb-DP-2021-003} &  {\small A comparison of CPU and GPU implementations for the LHCb \dots}\\
    \showcite{LHCb-DP-2021-002} &  {\small Centrality determination in heavy-ion collisions with the LHCb detector}\\
    \showcite{LHCb-DP-2021-001} &  {\small A parametrized Kalman filter for fast track fitting at LHCb}\\
    \showcite{LHCb-DP-2020-003} &  {\small Long-term operation of the multi-wire-proportional-chambers \dots}\\
    \showcite{LHCb-DP-2020-002} &  {\small Muon identification for LHCb Run 3}\\
    \showcite{LHCb-DP-2020-001} &  {\small Calibration and performance of the LHCb calorimeters in Run 1 and 2 \dots}\\
    \showcite{LHCb-DP-2019-004} &  {\small Real-time discrimination of photon pairs using machine learning \dots}\\
    \showcite{LHCb-DP-2019-003} &  {\small Measurement of the electron reconstruction efficiency at LHCb}\\
    \showcite{LHCb-DP-2019-002} &  {\small Real-Time analysis}\\
    \showcite{LHCb-DP-2019-001} &  {\small Run~2 trigger performance}\\
    \showcite{LHCb-DP-2018-004} &  {\small ReDecay}\\
    \showcite{LHCb-DP-2018-003} &  {\small Radiation damage in TT}\\
    \showcite{LHCb-DP-2018-002} &  {\small VeLo material map using SMOG}\\
    \showcite{LHCb-DP-2018-001} &  {\small PIDCalib for Run 2 (use Ref.~\cite{LHCb-PUB-2016-021} for Run~1)} \\
    \showcite{LHCb-DP-2017-001} &  {\small Performance of the Outer Tracker --- Run 2}\\
    \showcite{LHCb-DP-2016-003} &  {\small HeRSCheL} \\
    \showcite{LHCb-DP-2016-001} &  {\small TESLA project --- Run 2} \\
    \showcite{LHCb-DP-2014-002} &  {\small LHCb detector performance} \\
    \showcite{LHCb-DP-2014-001} &  {\small Performance of the LHCb Vertex Locator} \\
%%%    \showcite{LHCb-DP-2013-004} &  {\small Performance of the LHCb calorimeters} \\
    \showcite{LHCb-DP-2013-003} &  {\small Performance of the LHCb Outer Tracker --- Run 1} \\
    \showcite{LHCb-DP-2013-002} &  {\small Measurement of the track reconstruction efficiency at LHCb} \\
    \showcite{LHCb-DP-2013-001} &  {\small Performance of the muon identification at LHCb} \\
    \showcite{LHCb-DP-2012-005} &  {\small Radiation damage in the LHCb Vertex Locator} \\
    \showcite{LHCb-DP-2012-004} &  {\small The \lhcb trigger and its performance in 2011} \\
    \showcite{LHCb-DP-2012-003} &  {\small Performance of the \lhcb RICH detector at the LHC} \\
    \showcite{LHCb-DP-2012-002} &  {\small Performance of the LHCb muon system} \\
    \showcite{LHCb-DP-2012-001} &  {\small Radiation hardness of the LHCb Outer Tracker} \\
    \showcite{LHCb-DP-2011-002} &  {\small Simulation of machine induced background \dots} \\
    \showcite{LHCb-DP-2011-001} &  {\small Performance of the LHCb muon system with cosmic rays} \\
    \showcite{LHCb-DP-2010-001} &  {\small First spatial alignment of the LHCb VELO \dots} \\
    \showcite{LHCb-DP-2008-001} &  {\small \lhcb detector} \\
    \hline
  \end{longtable}
\end{center}

\begin{center}
\begin{longtable}{ll}
\caption{\small LHCb TDRs.}\label{tab:LHCb-TDRs}
\endfirsthead
\multicolumn{2}{c}{ -- continued from previous page.}
\endhead
\endfoot
\endlastfoot
    \hline
    \texttt{LHCb-TDR} number & Title \\
    \hline
    \showcite{LHCb-TDR-026} & {\small LHCb Upgrade II Scoping Document} \\
    \showcite{LHCb-TDR-025} & {\small LHCb Data Acquisition Enhancement Technical Design Report} \\
    \showcite{LHCb-TDR-024} & {\small LHCb Particle Identification Enhancement Technical Design Report} \\
    \showcite{LHCb-TDR-023} & {\small Framework TDR for LHCb Upgrade II} \\
    \showcite{LHCb-TDR-022} & {\small PLUME} \\
    \showcite{LHCb-TDR-021} & {\small Allen} \\
    \showcite{LHCb-TDR-020} & {\small SMOG Upgrade} \\
    \showcite{LHCb-TDR-018} & {\small Upgrade computing model} \\
    \showcite{LHCb-PII-Physics} & {\small Phase-II upgrade physics case} \\
    \showcite{LHCb-PII-EoI} & {\small Expression of interest for Phase-II upgrade} \\
    \showcite{LHCb-TDR-017} & {\small Upgrade software and computing} \\
    \showcite{LHCb-TDR-016} & {\small Trigger and online upgrade} \\
    \showcite{LHCb-TDR-015} & {\small Tracker upgrade} \\
    \showcite{LHCb-TDR-014} & {\small PID upgrade} \\
    \showcite{LHCb-TDR-013} & {\small VELO upgrade} \\
    \showcite{LHCb-TDR-012} & {\small Framework TDR for the upgrade} \\
    \showcite{LHCb-TDR-011} & {\small Computing} \\
    \showcite{LHCb-TDR-010} & {\small Trigger} \\
    \showcite{LHCb-TDR-009} & {\small Reoptimized detector} \\
    \showcite{LHCb-TDR-008} & {\small Inner Tracker} \\
    \showcite{LHCb-TDR-007} & {\small Online, DAQ, ECS} \\
    \showcite{LHCb-TDR-006} & {\small Outer Tracker} \\
    \showcite{LHCb-TDR-005} & {\small VELO} \\
    \showcite{LHCb-TDR-004} & {\small Muon system} \\
    \showcite{LHCb-TDR-003} & {\small RICH} \\
    \showcite{LHCb-TDR-002} & {\small Calorimeters} \\
    \showcite{LHCb-TDR-001} & {\small Magnet} \\
    \hline
  \end{longtable}
\end{center}

{\tiny\begin{center}
%  \begin{tabular}{l|l}
\begin{longtable}{lllll}
\caption{\small
  LHCb-PAPERs (which have their identifier as their cite code).
  DNE: Does not exist.
}
\label{tab:LHCb-PAPERs}
\endfirsthead
\multicolumn{5}{c}{ -- continued from previous page.}
\endhead
\endfoot
\endlastfoot

\showcite{LHCb-PAPER-2026-030}  & 
\showcite{LHCb-PAPER-2026-029} &
\showcite{LHCb-PAPER-2026-028}  &
\showcite{LHCb-PAPER-2026-027}  & 
\showcite{LHCb-PAPER-2026-026}  \\
\showcite{LHCb-PAPER-2026-025}  & 
\showcite{LHCb-PAPER-2026-024} &
\showcite{LHCb-PAPER-2026-023}  &
\showcite{LHCb-PAPER-2026-022}  & 
\showcite{LHCb-PAPER-2026-021}  \\
\showcite{LHCb-PAPER-2026-020}  & 
\showcite{LHCb-PAPER-2026-019} &
\showcite{LHCb-PAPER-2026-018}  &
\showcite{LHCb-PAPER-2026-017}  & 
\showcite{LHCb-PAPER-2026-016}  \\
\showcite{LHCb-PAPER-2026-015}  & 
\showcite{LHCb-PAPER-2026-014} &
\showcite{LHCb-PAPER-2026-013}  &
\showcite{LHCb-PAPER-2026-012}  & 
\showcite{LHCb-PAPER-2026-011}  \\
\showcite{LHCb-PAPER-2026-010}  & 
\showcite{LHCb-PAPER-2026-009} &
\showcite{LHCb-PAPER-2026-008}  &
\showcite{LHCb-PAPER-2026-007}  & 
\showcite{LHCb-PAPER-2026-006}  \\
\showcite{LHCb-PAPER-2026-005}  & 
\showcite{LHCb-PAPER-2026-004} &
\showcite{LHCb-PAPER-2026-003}  &
\showcite{LHCb-PAPER-2026-002}  & 
\showcite{LHCb-PAPER-2026-001}  \\
\hline
  & 
\showcite{LHCb-PAPER-2025-074} &
\showcite{LHCb-PAPER-2025-073}  &
\showcite{LHCb-PAPER-2025-072}  & 
\showcite{LHCb-PAPER-2025-071}  \\
\showcite{LHCb-PAPER-2025-070}  & 
\showcite{LHCb-PAPER-2025-069} &
\showcite{LHCb-PAPER-2025-068}  &
\showcite{LHCb-PAPER-2025-067}  & 
\showcite{LHCb-PAPER-2025-066}  \\
\showcite{LHCb-PAPER-2025-065}  & 
\showcite{LHCb-PAPER-2025-064} &
\showcite{LHCb-PAPER-2025-063}  &
\showcite{LHCb-PAPER-2025-062}  & 
\showcite{LHCb-PAPER-2025-061}  \\
\showcite{LHCb-PAPER-2025-060}  & 
\showcite{LHCb-PAPER-2025-059} &
\showcite{LHCb-PAPER-2025-058}  &
\showcite{LHCb-PAPER-2025-057}  & 
\showcite{LHCb-PAPER-2025-056}  \\
\showcite{LHCb-PAPER-2025-055}  & 
\showcite{LHCb-PAPER-2025-054} &
\showcite{LHCb-PAPER-2025-053}  &
\showcite{LHCb-PAPER-2025-052}  & 
\showcite{LHCb-PAPER-2025-051}  \\
\showcite{LHCb-PAPER-2025-050}  & 
\showcite{LHCb-PAPER-2025-049} &
\showcite{LHCb-PAPER-2025-048}  &
\showcite{LHCb-PAPER-2025-047}  & 
\showcite{LHCb-PAPER-2025-046}  \\
\showcite{LHCb-PAPER-2025-045}  & 
\showcite{LHCb-PAPER-2025-044} &
\showcite{LHCb-PAPER-2025-043}  &
\showcite{LHCb-PAPER-2025-042}  & 
\showcite{LHCb-PAPER-2025-041}  \\
\showcite{LHCb-PAPER-2025-040}  & 
\showcite{LHCb-PAPER-2025-039} &
\showcite{LHCb-PAPER-2025-038}  &
\showcite{LHCb-PAPER-2025-037}  & 
\showcite{LHCb-PAPER-2025-036}  \\
\showcite{LHCb-PAPER-2025-035}  & 
\showcite{LHCb-PAPER-2025-034} &
\showcite{LHCb-PAPER-2025-033}  &
\showcite{LHCb-PAPER-2025-032}  & 
\showcite{LHCb-PAPER-2025-031}  \\
\showcite{LHCb-PAPER-2025-030}  & 
\showcite{LHCb-PAPER-2025-029} &
\showcite{LHCb-PAPER-2025-028}  &
\showcite{LHCb-PAPER-2025-027}  & 
\showcite{LHCb-PAPER-2025-026}  \\
\showcite{LHCb-PAPER-2025-025}  & 
\showcite{LHCb-PAPER-2025-024} &
\showcite{LHCb-PAPER-2025-023}  &
\showcite{LHCb-PAPER-2025-022}  & 
\showcite{LHCb-PAPER-2025-021}  \\
\showcite{LHCb-PAPER-2025-020}  & 
\showcite{LHCb-PAPER-2025-019} &
\showcite{LHCb-PAPER-2025-018}  &
\showcite{LHCb-PAPER-2025-017}  & 
\showcite{LHCb-PAPER-2025-016}  \\
\showcite{LHCb-PAPER-2025-015}  & 
\showcite{LHCb-PAPER-2025-014} &
\showcite{LHCb-PAPER-2025-013}  &
\showcite{LHCb-PAPER-2025-012}  & 
\showcite{LHCb-PAPER-2025-011}  \\
\showcite{LHCb-PAPER-2025-010}  & 
\showcite{LHCb-PAPER-2025-009} &
\showcite{LHCb-PAPER-2025-008}  &
\showcite{LHCb-PAPER-2025-007}  & 
\showcite{LHCb-PAPER-2025-006}  \\
\showcite{LHCb-PAPER-2025-005}  & 
\showcite{LHCb-PAPER-2025-004} &
\showcite{LHCb-PAPER-2025-003}  &
\showcite{LHCb-PAPER-2025-002}  & 
\showcite{LHCb-PAPER-2025-001}  \\
\hline
\showcite{LHCb-PAPER-2024-056}  \\ 
\showcite{LHCb-PAPER-2024-055}  & 
\showcite{LHCb-PAPER-2024-054}  &
\showcite{LHCb-PAPER-2024-053}  &
\showcite{LHCb-PAPER-2024-052}  & 
\showcite{LHCb-PAPER-2024-051}  \\
\showcite{LHCb-PAPER-2024-050}  & 
\showcite{LHCb-PAPER-2024-049}  &
\showcite{LHCb-PAPER-2024-048}  &
\showcite{LHCb-PAPER-2024-047}  & 
\showcite{LHCb-PAPER-2024-046}  \\ 
\showcite{LHCb-PAPER-2024-045}  & 
\showcite{LHCb-PAPER-2024-044} &
\showcite{LHCb-PAPER-2024-043}  &
\showcite{LHCb-PAPER-2024-042}  & 
\showcite{LHCb-PAPER-2024-041}  \\ 
\showcite{LHCb-PAPER-2024-040} &
\showcite{LHCb-PAPER-2024-039} &
\showcite{LHCb-PAPER-2024-038}  &
\showcite{LHCb-PAPER-2024-037}  & 
\showcite{LHCb-PAPER-2024-036}  \\ 
\showcite{LHCb-PAPER-2024-035}  & 
\showcite{LHCb-PAPER-2024-034} &
\showcite{LHCb-PAPER-2024-033}  &
\showcite{LHCb-PAPER-2024-032}  & 
\showcite{LHCb-PAPER-2024-031}  \\ 
\showcite{LHCb-PAPER-2024-030} &
\showcite{LHCb-PAPER-2024-029} &
\showcite{LHCb-PAPER-2024-028}  &
\showcite{LHCb-PAPER-2024-027}  & 
\showcite{LHCb-PAPER-2024-026}  \\ 
\showcite{LHCb-PAPER-2024-025}  & 
\showcite{LHCb-PAPER-2024-024} &
\showcite{LHCb-PAPER-2024-023}  &
\showcite{LHCb-PAPER-2024-022}  & 
\showcite{LHCb-PAPER-2024-021}  \\ 
\showcite{LHCb-PAPER-2024-020} &
\showcite{LHCb-PAPER-2024-019} &
\showcite{LHCb-PAPER-2024-018}  &
\showcite{LHCb-PAPER-2024-017}  & 
\showcite{LHCb-PAPER-2024-016}  \\ 
\showcite{LHCb-PAPER-2024-015}  & 
\showcite{LHCb-PAPER-2024-014} &
\showcite{LHCb-PAPER-2024-013}  &
\showcite{LHCb-PAPER-2024-012}  & 
\showcite{LHCb-PAPER-2024-011} \\ 
\showcite{LHCb-PAPER-2024-010}  & 
\showcite{LHCb-PAPER-2024-009} &
\showcite{LHCb-PAPER-2024-008}  &
\showcite{LHCb-PAPER-2024-007}  & 
\showcite{LHCb-PAPER-2024-006}  \\ 
\showcite{LHCb-PAPER-2024-005}  &
\showcite{LHCb-PAPER-2024-004} &
\showcite{LHCb-PAPER-2024-003}  &
\showcite{LHCb-PAPER-2024-002}  & 
\showcite{LHCb-PAPER-2024-001}  \\
\hline
\showcite{LHCb-PAPER-2023-047}  & 
\showcite{LHCb-PAPER-2023-046} \\
\showcite{LHCb-PAPER-2023-045}  &
\showcite{LHCb-PAPER-2023-044}  & 
\showcite{LHCb-PAPER-2023-043}  & 
\showcite{LHCb-PAPER-2023-042}  & 
\showcite{LHCb-PAPER-2023-041} \\
\showcite{LHCb-PAPER-2023-040}  &
\showcite{LHCb-PAPER-2023-039}  & 
\showcite{LHCb-PAPER-2023-038}  & 
\showcite{LHCb-PAPER-2023-037}  & 
\showcite{LHCb-PAPER-2023-036} \\
\showcite{LHCb-PAPER-2023-035}  &
\showcite{LHCb-PAPER-2023-034}  & 
\showcite{LHCb-PAPER-2023-033}  & 
\showcite{LHCb-PAPER-2023-032}  & 
\showcite{LHCb-PAPER-2023-031} \\
\showcite{LHCb-PAPER-2023-030}  &
\showcite{LHCb-PAPER-2023-029}  & 
\showcite{LHCb-PAPER-2023-028}  & 
\showcite{LHCb-PAPER-2023-027}  & 
\showcite{LHCb-PAPER-2023-026} \\
\showcite{LHCb-PAPER-2023-025}  &
\showcite{LHCb-PAPER-2023-024}  & 
\showcite{LHCb-PAPER-2023-023}  & 
\showcite{LHCb-PAPER-2023-022}  & 
\showcite{LHCb-PAPER-2023-021} \\
\showcite{LHCb-PAPER-2023-020}  &
\showcite{LHCb-PAPER-2023-019}  & 
\showcite{LHCb-PAPER-2023-018}  & 
\showcite{LHCb-PAPER-2023-017}  & 
\showcite{LHCb-PAPER-2023-016} \\
\showcite{LHCb-PAPER-2023-015}  &
\showcite{LHCb-PAPER-2023-014}  & 
\showcite{LHCb-PAPER-2023-013}  & 
\showcite{LHCb-PAPER-2023-012}  & 
\showcite{LHCb-PAPER-2023-011} \\
\showcite{LHCb-PAPER-2023-010}  &
\showcite{LHCb-PAPER-2023-009}  & 
\showcite{LHCb-PAPER-2023-008}  & 
\showcite{LHCb-PAPER-2023-007}  & 
\showcite{LHCb-PAPER-2023-006} \\
\showcite{LHCb-PAPER-2023-005}  &
\showcite{LHCb-PAPER-2023-004}  & 
\showcite{LHCb-PAPER-2023-003}  & 
\showcite{LHCb-PAPER-2023-002}  & 
\showcite{LHCb-PAPER-2023-001} \\
\hline
  &
\showcite{LHCb-PAPER-2022-054}  &
\showcite{LHCb-PAPER-2022-053}  &
\showcite{LHCb-PAPER-2022-052}  &
\showcite{LHCb-PAPER-2022-051} \\
\showcite{LHCb-PAPER-2022-050}  &
\showcite{LHCb-PAPER-2022-049}  &
\showcite{LHCb-PAPER-2022-048}  &
\showcite{LHCb-PAPER-2022-047}  &
\showcite{LHCb-PAPER-2022-046} \\
\showcite{LHCb-PAPER-2022-045}  &
\showcite{LHCb-PAPER-2022-044}  &
\showcite{LHCb-PAPER-2022-043}  &
\showcite{LHCb-PAPER-2022-042}  &
\showcite{LHCb-PAPER-2022-041} \\
\showcite{LHCb-PAPER-2022-040}  &
\showcite{LHCb-PAPER-2022-039}  &
\showcite{LHCb-PAPER-2022-038}  &
\showcite{LHCb-PAPER-2022-037}  &
\showcite{LHCb-PAPER-2022-036} \\
\showcite{LHCb-PAPER-2022-035}  &
\showcite{LHCb-PAPER-2022-034}  &
\showcite{LHCb-PAPER-2022-033}  &
\showcite{LHCb-PAPER-2022-032}  &
\showcite{LHCb-PAPER-2022-031} \\
\showcite{LHCb-PAPER-2022-030}  &
\showcite{LHCb-PAPER-2022-029}  &
\showcite{LHCb-PAPER-2022-028}  &
\showcite{LHCb-PAPER-2022-027}  &
\showcite{LHCb-PAPER-2022-026} \\
\showcite{LHCb-PAPER-2022-025}  &
\showcite{LHCb-PAPER-2022-024}  &
\showcite{LHCb-PAPER-2022-023}  &
\showcite{LHCb-PAPER-2022-022}  &
\showcite{LHCb-PAPER-2022-021} \\
\showcite{LHCb-PAPER-2022-020}  &
\showcite{LHCb-PAPER-2022-019}  &
\showcite{LHCb-PAPER-2022-018}  &
\showcite{LHCb-PAPER-2022-017}  &
\showcite{LHCb-PAPER-2022-016} \\
\showcite{LHCb-PAPER-2022-015}  &
\showcite{LHCb-PAPER-2022-014}  &
\showcite{LHCb-PAPER-2022-013}  &
\showcite{LHCb-PAPER-2022-012}  &
\showcite{LHCb-PAPER-2022-011}  \\
\showcite{LHCb-PAPER-2022-010}  &
\showcite{LHCb-PAPER-2022-009}  &
\showcite{LHCb-PAPER-2022-008}  &
\showcite{LHCb-PAPER-2022-007}  &
\showcite{LHCb-PAPER-2022-006} \\
\showcite{LHCb-PAPER-2022-005}  &
\showcite{LHCb-PAPER-2022-004}  &
\showcite{LHCb-PAPER-2022-003}  &
\showcite{LHCb-PAPER-2022-002}  &
\showcite{LHCb-PAPER-2022-001}  \\
\hline
\showcite{LHCb-PAPER-2021-053}  &
\showcite{LHCb-PAPER-2021-052}  &
\showcite{LHCb-PAPER-2021-051} \\
\showcite{LHCb-PAPER-2021-050}  &
\showcite{LHCb-PAPER-2021-049}  &
\showcite{LHCb-PAPER-2021-048}  &
\showcite{LHCb-PAPER-2021-047}  &
\showcite{LHCb-PAPER-2021-046} \\
\showcite{LHCb-PAPER-2021-045}  &
\showcite{LHCb-PAPER-2021-044}  &
\showcite{LHCb-PAPER-2021-043}  &
\showcite{LHCb-PAPER-2021-042}  &
\showcite{LHCb-PAPER-2021-041} \\
\showcite{LHCb-PAPER-2021-040}  &
\showcite{LHCb-PAPER-2021-039}  &
\showcite{LHCb-PAPER-2021-038}  &
\showcite{LHCb-PAPER-2021-037}  &
\showcite{LHCb-PAPER-2021-036} \\
\showcite{LHCb-PAPER-2021-035}  &
\showcite{LHCb-PAPER-2021-034}  &
\showcite{LHCb-PAPER-2021-033}  &
\showcite{LHCb-PAPER-2021-032}  &
\showcite{LHCb-PAPER-2021-031} \\
\showcite{LHCb-PAPER-2021-030}  &
\showcite{LHCb-PAPER-2021-029}  &
\showcite{LHCb-PAPER-2021-028}  &
\showcite{LHCb-PAPER-2021-027}  &
\showcite{LHCb-PAPER-2021-026} \\
\showcite{LHCb-PAPER-2021-025}  &
\showcite{LHCb-PAPER-2021-024}  &
\showcite{LHCb-PAPER-2021-023}  &
\showcite{LHCb-PAPER-2021-022}  &
\showcite{LHCb-PAPER-2021-021} \\
\showcite{LHCb-PAPER-2021-020}  &
\showcite{LHCb-PAPER-2021-019}  &
\showcite{LHCb-PAPER-2021-018}  &
\showcite{LHCb-PAPER-2021-017}  &
\showcite{LHCb-PAPER-2021-016} \\
\showcite{LHCb-PAPER-2021-015}  &
\showcite{LHCb-PAPER-2021-014}  &
\showcite{LHCb-PAPER-2021-013}  &
\showcite{LHCb-PAPER-2021-012}  &
\showcite{LHCb-PAPER-2021-011} \\
\showcite{LHCb-PAPER-2021-010}  &
\showcite{LHCb-PAPER-2021-009}  &
\showcite{LHCb-PAPER-2021-008}  &
\showcite{LHCb-PAPER-2021-007}  &
\showcite{LHCb-PAPER-2021-006} \\
\showcite{LHCb-PAPER-2021-005}  &
\showcite{LHCb-PAPER-2021-004}  &
\showcite{LHCb-PAPER-2021-003}  &
\showcite{LHCb-PAPER-2021-002}  &
\showcite{LHCb-PAPER-2021-001} \\
\hline
\showcite{LHCb-PAPER-2020-048}  &
\showcite{LHCb-PAPER-2020-047}  &
\showcite{LHCb-PAPER-2020-046}  \\
\showcite{LHCb-PAPER-2020-045}  &
\showcite{LHCb-PAPER-2020-044}  &
\showcite{LHCb-PAPER-2020-043}  &
\showcite{LHCb-PAPER-2020-042}  &
\showcite{LHCb-PAPER-2020-041} \\
\showcite{LHCb-PAPER-2020-040}  &
\showcite{LHCb-PAPER-2020-039}  &
\showcite{LHCb-PAPER-2020-038}  &
\showcite{LHCb-PAPER-2020-037}  &
\showcite{LHCb-PAPER-2020-036} \\
\showcite{LHCb-PAPER-2020-035}  &
\showcite{LHCb-PAPER-2020-034}  &
\showcite{LHCb-PAPER-2020-033}  &
\showcite{LHCb-PAPER-2020-032}  &
\showcite{LHCb-PAPER-2020-031} \\
\showcite{LHCb-PAPER-2020-030}  &
\showcite{LHCb-PAPER-2020-029}  &
\showcite{LHCb-PAPER-2020-028}  &
\showcite{LHCb-PAPER-2020-027}  &
\showcite{LHCb-PAPER-2020-026} \\
\showcite{LHCb-PAPER-2020-025}  &
\showcite{LHCb-PAPER-2020-024}  &
\showcite{LHCb-PAPER-2020-023}  &
\showcite{LHCb-PAPER-2020-022}  &
\showcite{LHCb-PAPER-2020-021} \\
\showcite{LHCb-PAPER-2020-020}  &
\showcite{LHCb-PAPER-2020-019}  &
\showcite{LHCb-PAPER-2020-018}  &
\showcite{LHCb-PAPER-2020-017}  &
\showcite{LHCb-PAPER-2020-016} \\
\showcite{LHCb-PAPER-2020-015}  &
\showcite{LHCb-PAPER-2020-014}  &
\showcite{LHCb-PAPER-2020-013}  &
\showcite{LHCb-PAPER-2020-012}  &
\showcite{LHCb-PAPER-2020-011} \\
\showcite{LHCb-PAPER-2020-010}  &
\showcite{LHCb-PAPER-2020-009}  &
\showcite{LHCb-PAPER-2020-008}  &
\showcite{LHCb-PAPER-2020-007}  &
\showcite{LHCb-PAPER-2020-006} \\
\showcite{LHCb-PAPER-2020-005}  &
\showcite{LHCb-PAPER-2020-004}  &
\showcite{LHCb-PAPER-2020-003}  &
\showcite{LHCb-PAPER-2020-002}  &
\showcite{LHCb-PAPER-2020-001} \\
\hline
\showcite{LHCb-PAPER-2019-046} \\
\showcite{LHCb-PAPER-2019-045}  &
\showcite{LHCb-PAPER-2019-044}  &
\showcite{LHCb-PAPER-2019-043}  &
\showcite{LHCb-PAPER-2019-042}  &
\showcite{LHCb-PAPER-2019-041} \\
\showcite{LHCb-PAPER-2019-040}  &
\showcite{LHCb-PAPER-2019-039}  &
\showcite{LHCb-PAPER-2019-038}  &
\showcite{LHCb-PAPER-2019-037}  &
\showcite{LHCb-PAPER-2019-036} \\
\showcite{LHCb-PAPER-2019-035}  &
\showcite{LHCb-PAPER-2019-034}  &
\showcite{LHCb-PAPER-2019-033}  &
\showcite{LHCb-PAPER-2019-032}  &
\showcite{LHCb-PAPER-2019-031} \\
\showcite{LHCb-PAPER-2019-030}  &
\showcite{LHCb-PAPER-2019-029}  &
\showcite{LHCb-PAPER-2019-028}  &
\showcite{LHCb-PAPER-2019-027}  &
\showcite{LHCb-PAPER-2019-026} \\
\showcite{LHCb-PAPER-2019-025}  &
\showcite{LHCb-PAPER-2019-024}  &
\showcite{LHCb-PAPER-2019-023}  &
\showcite{LHCb-PAPER-2019-022}  &
\showcite{LHCb-PAPER-2019-021} \\
\showcite{LHCb-PAPER-2019-020}  &
\showcite{LHCb-PAPER-2019-019}  &
\showcite{LHCb-PAPER-2019-018}  &
\showcite{LHCb-PAPER-2019-017}  &
\showcite{LHCb-PAPER-2019-016} \\
\showcite{LHCb-PAPER-2019-015}  &
\showcite{LHCb-PAPER-2019-014}  &
\showcite{LHCb-PAPER-2019-013}  &
\showcite{LHCb-PAPER-2019-012}  &
\showcite{LHCb-PAPER-2019-011} \\
\showcite{LHCb-PAPER-2019-010}  &
\showcite{LHCb-PAPER-2019-009}  &
\showcite{LHCb-PAPER-2019-008}  &
\showcite{LHCb-PAPER-2019-007}  &
\showcite{LHCb-PAPER-2019-006} \\
\showcite{LHCb-PAPER-2019-005}  &
\showcite{LHCb-PAPER-2019-004}  &
\showcite{LHCb-PAPER-2019-003}  &
\showcite{LHCb-PAPER-2019-002}  &
\showcite{LHCb-PAPER-2019-001} \\
\hline
\showcite{LHCb-PAPER-2018-051} \\
\showcite{LHCb-PAPER-2018-050}  &
\showcite{LHCb-PAPER-2018-049}  &
\showcite{LHCb-PAPER-2018-048}  &
\showcite{LHCb-PAPER-2018-047}  &
\showcite{LHCb-PAPER-2018-046} \\
\showcite{LHCb-PAPER-2018-045}  &
\showcite{LHCb-PAPER-2018-044}  &
\showcite{LHCb-PAPER-2018-043}  &
\showcite{LHCb-PAPER-2018-042}  &
\showcite{LHCb-PAPER-2018-041} \\
\showcite{LHCb-PAPER-2018-040}  &
\showcite{LHCb-PAPER-2018-039}  &
\showcite{LHCb-PAPER-2018-038}  &
\showcite{LHCb-PAPER-2018-037}  &
\showcite{LHCb-PAPER-2018-036} \\
\showcite{LHCb-PAPER-2018-035}  &
\showcite{LHCb-PAPER-2018-034}  &
\showcite{LHCb-PAPER-2018-033}  &
\showcite{LHCb-PAPER-2018-032}  &
\showcite{LHCb-PAPER-2018-031} \\
\showcite{LHCb-PAPER-2018-030}  &
\showcite{LHCb-PAPER-2018-029}  &
\showcite{LHCb-PAPER-2018-028}  &
\showcite{LHCb-PAPER-2018-027}  &
\showcite{LHCb-PAPER-2018-026} \\
\showcite{LHCb-PAPER-2018-025}  &
\showcite{LHCb-PAPER-2018-024}  &
\showcite{LHCb-PAPER-2018-023}  &
\showcite{LHCb-PAPER-2018-022}  &
\showcite{LHCb-PAPER-2018-021} \\
\showcite{LHCb-PAPER-2018-020}  &
\showcite{LHCb-PAPER-2018-019}  &
\showcite{LHCb-PAPER-2018-018}  &
\showcite{LHCb-PAPER-2018-017}  &
\showcite{LHCb-PAPER-2018-016} \\
\showcite{LHCb-PAPER-2018-015}  &
\showcite{LHCb-PAPER-2018-014}  &
\showcite{LHCb-PAPER-2018-013}  &
\showcite{LHCb-PAPER-2018-012}  &
\showcite{LHCb-PAPER-2018-011} \\
\showcite{LHCb-PAPER-2018-010}  &
\showcite{LHCb-PAPER-2018-009}  &
\showcite{LHCb-PAPER-2018-008}  &
\showcite{LHCb-PAPER-2018-007}  &
\showcite{LHCb-PAPER-2018-006} \\
\showcite{LHCb-PAPER-2018-005}  &
\showcite{LHCb-PAPER-2018-004}  &
\showcite{LHCb-PAPER-2018-003}  &
\showcite{LHCb-PAPER-2018-002}  &
\showcite{LHCb-PAPER-2018-001} \\
\hline 
\showcite{LHCb-PAPER-2017-050}  &
\showcite{LHCb-PAPER-2017-049}  &
\showcite{LHCb-PAPER-2017-048}  &
\showcite{LHCb-PAPER-2017-047}  &
\showcite{LHCb-PAPER-2017-046} \\
\showcite{LHCb-PAPER-2017-045}  &
\showcite{LHCb-PAPER-2017-044}  &
\showcite{LHCb-PAPER-2017-043}  &
\showcite{LHCb-PAPER-2017-042}  &
\showcite{LHCb-PAPER-2017-041} \\
\showcite{LHCb-PAPER-2017-040}  &
\showcite{LHCb-PAPER-2017-039}  &
\showcite{LHCb-PAPER-2017-038}  &
\showcite{LHCb-PAPER-2017-037}  &
\showcite{LHCb-PAPER-2017-036} \\
\showcite{LHCb-PAPER-2017-035}  &
\showcite{LHCb-PAPER-2017-034}  &
\showcite{LHCb-PAPER-2017-033}  &
\showcite{LHCb-PAPER-2017-032}  &
\showcite{LHCb-PAPER-2017-031} \\
\showcite{LHCb-PAPER-2017-030}  &
\showcite{LHCb-PAPER-2017-029}  &
\showcite{LHCb-PAPER-2017-028}  &
\showcite{LHCb-PAPER-2017-027}  &
\showcite{LHCb-PAPER-2017-026} \\
\showcite{LHCb-PAPER-2017-025}  &
\showcite{LHCb-PAPER-2017-024}  &
\showcite{LHCb-PAPER-2017-023}  &
\showcite{LHCb-PAPER-2017-022}  &
\showcite{LHCb-PAPER-2017-021} \\
\showcite{LHCb-PAPER-2017-020}  &
\showcite{LHCb-PAPER-2017-019}  &
\showcite{LHCb-PAPER-2017-018}  &
\showcite{LHCb-PAPER-2017-017}  &
\showcite{LHCb-PAPER-2017-016} \\
\showcite{LHCb-PAPER-2017-015}  &
\showcite{LHCb-PAPER-2017-014}  &
\showcite{LHCb-PAPER-2017-013}  &
\showcite{LHCb-PAPER-2017-012}  &
\showcite{LHCb-PAPER-2017-011} \\
\showcite{LHCb-PAPER-2017-010}  &
\showcite{LHCb-PAPER-2017-009}  &
\showcite{LHCb-PAPER-2017-008}  &
\showcite{LHCb-PAPER-2017-007}  &
\showcite{LHCb-PAPER-2017-006} \\
\showcite{LHCb-PAPER-2017-005}  &
\showcite{LHCb-PAPER-2017-004}  &
\showcite{LHCb-PAPER-2017-003}  &
\showcite{LHCb-PAPER-2017-002}  &
\showcite{LHCb-PAPER-2017-001} \\
\hline 
\showcite{LHCb-PAPER-2016-065}  &
\showcite{LHCb-PAPER-2016-064}  &
\showcite{LHCb-PAPER-2016-063}  &
\showcite{LHCb-PAPER-2016-062}  &
\showcite{LHCb-PAPER-2016-061} \\
\showcite{LHCb-PAPER-2016-060}  &
\showcite{LHCb-PAPER-2016-059}  &
\showcite{LHCb-PAPER-2016-058}  &
\showcite{LHCb-PAPER-2016-057}  &
\showcite{LHCb-PAPER-2016-056} \\
\showcite{LHCb-PAPER-2016-055}  &
\showcite{LHCb-PAPER-2016-054}  &
\showcite{LHCb-PAPER-2016-053}  &
\showcite{LHCb-PAPER-2016-052}  &
\showcite{LHCb-PAPER-2016-051} \\
\showcite{LHCb-PAPER-2016-050}  &
\showcite{LHCb-PAPER-2016-049}  &
\showcite{LHCb-PAPER-2016-048}  &
\showcite{LHCb-PAPER-2016-047}  &
\showcite{LHCb-PAPER-2016-046} \\
\showcite{LHCb-PAPER-2016-045}  &
\showcite{LHCb-PAPER-2016-044}  &
\showcite{LHCb-PAPER-2016-043}  &
\showcite{LHCb-PAPER-2016-042}  &
\showcite{LHCb-PAPER-2016-041} \\
\showcite{LHCb-PAPER-2016-040}  &
\showcite{LHCb-PAPER-2016-039}  &
\showcite{LHCb-PAPER-2016-038}  &
\showcite{LHCb-PAPER-2016-037}  &
\showcite{LHCb-PAPER-2016-036} \\
\showcite{LHCb-PAPER-2016-035}  &
\showcite{LHCb-PAPER-2016-034}  &
\showcite{LHCb-PAPER-2016-033}  &
\showcite{LHCb-PAPER-2016-032}  &
\showcite{LHCb-PAPER-2016-031} \\
\showcite{LHCb-PAPER-2016-030}  &
\showcite{LHCb-PAPER-2016-029}  &
\showcite{LHCb-PAPER-2016-028}  &
\showcite{LHCb-PAPER-2016-027}  &
\showcite{LHCb-PAPER-2016-026} \\
\showcite{LHCb-PAPER-2016-025}  &
\showcite{LHCb-PAPER-2016-024}  &
\showcite{LHCb-PAPER-2016-023}  &
\showcite{LHCb-PAPER-2016-022}  &
\showcite{LHCb-PAPER-2016-021} \\
\showcite{LHCb-PAPER-2016-020}  &
\showcite{LHCb-PAPER-2016-019}  &
\showcite{LHCb-PAPER-2016-018}  &
\showcite{LHCb-PAPER-2016-017}  &
\showcite{LHCb-PAPER-2016-016} \\
\showcite{LHCb-PAPER-2016-015}  &
\showcite{LHCb-PAPER-2016-014}  &
\showcite{LHCb-PAPER-2016-013}  &
\showcite{LHCb-PAPER-2016-012}  &
\showcite{LHCb-PAPER-2016-011} \\
\showcite{LHCb-PAPER-2016-010}  &
\showcite{LHCb-PAPER-2016-009}  &
\showcite{LHCb-PAPER-2016-008}  &
\showcite{LHCb-PAPER-2016-007}  &
\showcite{LHCb-PAPER-2016-006} \\
\showcite{LHCb-PAPER-2016-005}  &
\showcite{LHCb-PAPER-2016-004}  &
\showcite{LHCb-PAPER-2016-003}  &
\showcite{LHCb-PAPER-2016-002}  &
\showcite{LHCb-PAPER-2016-001} \\
\hline
\showcite{LHCb-PAPER-2015-060}  &
\showcite{LHCb-PAPER-2015-059}  &
\showcite{LHCb-PAPER-2015-058}  &
\showcite{LHCb-PAPER-2015-057}  &
\showcite{LHCb-PAPER-2015-056} \\
\showcite{LHCb-PAPER-2015-055}  &
\showcite{LHCb-PAPER-2015-054}  &
\showcite{LHCb-PAPER-2015-053}  &
\showcite{LHCb-PAPER-2015-052}  &
\showcite{LHCb-PAPER-2015-051} \\
\showcite{LHCb-PAPER-2015-050}  &
\showcite{LHCb-PAPER-2015-049}  &
\showcite{LHCb-PAPER-2015-048}  &
\showcite{LHCb-PAPER-2015-047}  &
\showcite{LHCb-PAPER-2015-046} \\
\showcite{LHCb-PAPER-2015-045}  &
\showcite{LHCb-PAPER-2015-044}  &
\showcite{LHCb-PAPER-2015-043}  &
\showcite{LHCb-PAPER-2015-042}  &
\showcite{LHCb-PAPER-2015-041} \\
\showcite{LHCb-PAPER-2015-040}  &
\showcite{LHCb-PAPER-2015-039}  &
\showcite{LHCb-PAPER-2015-038}  &
\showcite{LHCb-PAPER-2015-037}  &
\showcite{LHCb-PAPER-2015-036} \\
\showcite{LHCb-PAPER-2015-035}  &
\showcite{LHCb-PAPER-2015-034}  &
\showcite{LHCb-PAPER-2015-033}  &
\showcite{LHCb-PAPER-2015-032}  &
\showcite{LHCb-PAPER-2015-031} \\
\showcite{LHCb-PAPER-2015-030}  &
\showcite{LHCb-PAPER-2015-029}  &
\showcite{LHCb-PAPER-2015-028}  &
\showcite{LHCb-PAPER-2015-027}  &
\showcite{LHCb-PAPER-2015-026} \\
\showcite{LHCb-PAPER-2015-025}  &
\showcite{LHCb-PAPER-2015-024}  &
\showcite{LHCb-PAPER-2015-023}  &
\showcite{LHCb-PAPER-2015-022}  &
\showcite{LHCb-PAPER-2015-021} \\
\showcite{LHCb-PAPER-2015-020}  &
\showcite{LHCb-PAPER-2015-019}  &
\showcite{LHCb-PAPER-2015-018}  &
\showcite{LHCb-PAPER-2015-017}  &
\showcite{LHCb-PAPER-2015-016} \\
\showcite{LHCb-PAPER-2015-015}  &
\showcite{LHCb-PAPER-2015-014}  &
\showcite{LHCb-PAPER-2015-013}  &
\showcite{LHCb-PAPER-2015-012}  &
\showcite{LHCb-PAPER-2015-011} \\
\showcite{LHCb-PAPER-2015-010}  &
\showcite{LHCb-PAPER-2015-009}  &
\showcite{LHCb-PAPER-2015-008}  &
\showcite{LHCb-PAPER-2015-007}  &
\showcite{LHCb-PAPER-2015-006} \\
\showcite{LHCb-PAPER-2015-005}  &
\showcite{LHCb-PAPER-2015-004}  &
\showcite{LHCb-PAPER-2015-003}  &
\showcite{LHCb-PAPER-2015-002}  &
\showcite{LHCb-PAPER-2015-001} \\
\hline 
\showcite{LHCb-PAPER-2014-070}  &
\showcite{LHCb-PAPER-2014-069}  &
\showcite{LHCb-PAPER-2014-068}  &
\showcite{LHCb-PAPER-2014-067}  &
\showcite{LHCb-PAPER-2014-066} \\
\showcite{LHCb-PAPER-2014-065}  &
\showcite{LHCb-PAPER-2014-064}  &
\showcite{LHCb-PAPER-2014-063}  &
\showcite{LHCb-PAPER-2014-062}  &
\showcite{LHCb-PAPER-2014-061} \\
\showcite{LHCb-PAPER-2014-060}  &
\showcite{LHCb-PAPER-2014-059}  &
\showcite{LHCb-PAPER-2014-058}  &
\showcite{LHCb-PAPER-2014-057}  &
\showcite{LHCb-PAPER-2014-056} \\
\showcite{LHCb-PAPER-2014-055}  &
\showcite{LHCb-PAPER-2014-054}  &
\showcite{LHCb-PAPER-2014-053}  &
\showcite{LHCb-PAPER-2014-052}  &
\showcite{LHCb-PAPER-2014-051} \\
\showcite{LHCb-PAPER-2014-050}  &
\showcite{LHCb-PAPER-2014-049}  &
\showcite{LHCb-PAPER-2014-048}  &
\showcite{LHCb-PAPER-2014-047}  &
\showcite{LHCb-PAPER-2014-046} \\
\showcite{LHCb-PAPER-2014-045}  &
\showcite{LHCb-PAPER-2014-044}  &
\showcite{LHCb-PAPER-2014-043}  &
\showcite{LHCb-PAPER-2014-042}  &
\showcite{LHCb-PAPER-2014-041} \\
\showcite{LHCb-PAPER-2014-040}  &
\showcite{LHCb-PAPER-2014-039}  &
\showcite{LHCb-PAPER-2014-038}  &
\showcite{LHCb-PAPER-2014-037}  &
\showcite{LHCb-PAPER-2014-036} \\
\showcite{LHCb-PAPER-2014-035}  &
\showcite{LHCb-PAPER-2014-034}  &
\showcite{LHCb-PAPER-2014-033}  &
\showcite{LHCb-PAPER-2014-032}  &
\showcite{LHCb-PAPER-2014-031} \\
\showcite{LHCb-PAPER-2014-030}  &
\showcite{LHCb-PAPER-2014-029}  &
\showcite{LHCb-PAPER-2014-028}  &
\showcite{LHCb-PAPER-2014-027}  &
\showcite{LHCb-PAPER-2014-026} \\
\showcite{LHCb-PAPER-2014-025}  &
\showcite{LHCb-PAPER-2014-024}  &
\showcite{LHCb-PAPER-2014-023}  &
\showcite{LHCb-PAPER-2014-022}  &
\showcite{LHCb-PAPER-2014-021} \\
\showcite{LHCb-PAPER-2014-020}  &
\showcite{LHCb-PAPER-2014-019}  &
\showcite{LHCb-PAPER-2014-018}  &
\showcite{LHCb-PAPER-2014-017}  &
\showcite{LHCb-PAPER-2014-016} \\
\showcite{LHCb-PAPER-2014-015}  &
\showcite{LHCb-PAPER-2014-014}  &
\showcite{LHCb-PAPER-2014-013}  &
\showcite{LHCb-PAPER-2014-012}  &
\showcite{LHCb-PAPER-2014-011} \\
\showcite{LHCb-PAPER-2014-010}  &
\showcite{LHCb-PAPER-2014-009}  &
\showcite{LHCb-PAPER-2014-008}  &
\showcite{LHCb-PAPER-2014-007}  &
\showcite{LHCb-PAPER-2014-006} \\
\showcite{LHCb-PAPER-2014-005}  &
\showcite{LHCb-PAPER-2014-004}  &
\showcite{LHCb-PAPER-2014-003}  &
\showcite{LHCb-PAPER-2014-002}  &
\showcite{LHCb-PAPER-2014-001} \\
\hline 
\showcite{LHCb-PAPER-2013-070}  &
\showcite{LHCb-PAPER-2013-069}  &
\showcite{LHCb-PAPER-2013-068}  &
\showcite{LHCb-PAPER-2013-067}  &
\showcite{LHCb-PAPER-2013-066} \\
\showcite{LHCb-PAPER-2013-065}  &
\showcite{LHCb-PAPER-2013-064}  &
\showcite{LHCb-PAPER-2013-063}  &
\showcite{LHCb-PAPER-2013-062}  &
\showcite{LHCb-PAPER-2013-061} \\
\showcite{LHCb-PAPER-2013-060}  &
\showcite{LHCb-PAPER-2013-059}  &
\showcite{LHCb-PAPER-2013-058}  &
\showcite{LHCb-PAPER-2013-057}  &
\showcite{LHCb-PAPER-2013-056} \\
\showcite{LHCb-PAPER-2013-055}  &
\showcite{LHCb-PAPER-2013-054}  &
\showcite{LHCb-PAPER-2013-053}  &
\showcite{LHCb-PAPER-2013-052}  &
\showcite{LHCb-PAPER-2013-051} \\
\showcite{LHCb-PAPER-2013-050}  &
\showcite{LHCb-PAPER-2013-049}  &
\showcite{LHCb-PAPER-2013-048}  &
\showcite{LHCb-PAPER-2013-047}  &
\showcite{LHCb-PAPER-2013-046} \\
\showcite{LHCb-PAPER-2013-045}  &
\showcite{LHCb-PAPER-2013-044}  &
\showcite{LHCb-PAPER-2013-043}  &
\showcite{LHCb-PAPER-2013-042}  &
\showcite{LHCb-PAPER-2013-041} \\
\showcite{LHCb-PAPER-2013-040}  &
\showcite{LHCb-PAPER-2013-039}  &
\showcite{LHCb-PAPER-2013-038}  &
\showcite{LHCb-PAPER-2013-037}  &
\showcite{LHCb-PAPER-2013-036} \\
\showcite{LHCb-PAPER-2013-035}  &
\showcite{LHCb-PAPER-2013-034}  &
\showcite{LHCb-PAPER-2013-033}  &
\showcite{LHCb-PAPER-2013-032}  &
\showcite{LHCb-PAPER-2013-031} \\
\showcite{LHCb-PAPER-2013-030}  &
\showcite{LHCb-PAPER-2013-029}  &
\showcite{LHCb-PAPER-2013-028}  &
\showcite{LHCb-PAPER-2013-027}  &
\showcite{LHCb-PAPER-2013-026} \\
\showcite{LHCb-PAPER-2013-025}  &
\showcite{LHCb-PAPER-2013-024}  &
\showcite{LHCb-PAPER-2013-023}  &
\showcite{LHCb-PAPER-2013-022}  &
\showcite{LHCb-PAPER-2013-021} \\
\showcite{LHCb-PAPER-2013-020}  &
\showcite{LHCb-PAPER-2013-019}  &
\showcite{LHCb-PAPER-2013-018}  &
\showcite{LHCb-PAPER-2013-017}  &
\showcite{LHCb-PAPER-2013-016} \\
\showcite{LHCb-PAPER-2013-015}  &
\showcite{LHCb-PAPER-2013-014}  &
\showcite{LHCb-PAPER-2013-013}  &
\showcite{LHCb-PAPER-2013-012}  &
\showcite{LHCb-PAPER-2013-011} \\
\showcite{LHCb-PAPER-2013-010}  &
\showcite{LHCb-PAPER-2013-009}  &
\showcite{LHCb-PAPER-2013-008}  &
\showcite{LHCb-PAPER-2013-007}  &
\showcite{LHCb-PAPER-2013-006} \\
\showcite{LHCb-PAPER-2013-005}  &
\showcite{LHCb-PAPER-2013-004}  &
\showcite{LHCb-PAPER-2013-003}  &
\showcite{LHCb-PAPER-2013-002}  &
\showcite{LHCb-PAPER-2013-001} \\
\hline
\showcite{LHCb-PAPER-2012-057}  &
\showcite{LHCb-PAPER-2012-056} \\
\showcite{LHCb-PAPER-2012-055}  &
\showcite{LHCb-PAPER-2012-054}  &
\showcite{LHCb-PAPER-2012-053}  &
\showcite{LHCb-PAPER-2012-052}  &
\showcite{LHCb-PAPER-2012-051} \\
\showcite{LHCb-PAPER-2012-050}  &
\showcite{LHCb-PAPER-2012-049}  &
\showcite{LHCb-PAPER-2012-048}  &
\showcite{LHCb-PAPER-2012-047}  &
\showcite{LHCb-PAPER-2012-046} \\
\showcite{LHCb-PAPER-2012-045}  &
\showcite{LHCb-PAPER-2012-044}  &
\showcite{LHCb-PAPER-2012-043}  &
\showcite{LHCb-PAPER-2012-042}  &
\showcite{LHCb-PAPER-2012-041} \\
\showcite{LHCb-PAPER-2012-040}  &
\showcite{LHCb-PAPER-2012-039}  &
\showcite{LHCb-PAPER-2012-038}  &
\showcite{LHCb-PAPER-2012-037}  &
\showcite{LHCb-PAPER-2012-036} \\
\showcite{LHCb-PAPER-2012-035}  &
\showcite{LHCb-PAPER-2012-034}  &
\showcite{LHCb-PAPER-2012-033}  &
\showcite{LHCb-PAPER-2012-032}  &
\showcite{LHCb-PAPER-2012-031} \\
\showcite{LHCb-PAPER-2012-030}  &
\showcite{LHCb-PAPER-2012-029}  &
\showcite{LHCb-PAPER-2012-028}  &
\showcite{LHCb-PAPER-2012-027}  &
\showcite{LHCb-PAPER-2012-026} \\
\showcite{LHCb-PAPER-2012-025}  &
\showcite{LHCb-PAPER-2012-024}  &
\showcite{LHCb-PAPER-2012-023}  &
\showcite{LHCb-PAPER-2012-022}  &
\showcite{LHCb-PAPER-2012-021} \\
\showcite{LHCb-PAPER-2012-020}  &
\showcite{LHCb-PAPER-2012-019}  &
\showcite{LHCb-PAPER-2012-018}  &
\showcite{LHCb-PAPER-2012-017}  &
\showcite{LHCb-PAPER-2012-016} \\
\showcite{LHCb-PAPER-2012-015}  &
\showcite{LHCb-PAPER-2012-014}  &
\showcite{LHCb-PAPER-2012-013}  &
\showcite{LHCb-PAPER-2012-012}  &
\showcite{LHCb-PAPER-2012-011} \\
\showcite{LHCb-PAPER-2012-010}  &
\showcite{LHCb-PAPER-2012-009}  &
\showcite{LHCb-PAPER-2012-008}  &
\showcite{LHCb-PAPER-2012-007}  &
\showcite{LHCb-PAPER-2012-006} \\
\showcite{LHCb-PAPER-2012-005}  &
\showcite{LHCb-PAPER-2012-004}  &
\showcite{LHCb-PAPER-2012-003}  &
\showcite{LHCb-PAPER-2012-002}  &
\showcite{LHCb-PAPER-2012-001} \\
\hline
\showcite{LHCb-PAPER-2011-045}  &
\showcite{LHCb-PAPER-2011-044}  &
\showcite{LHCb-PAPER-2011-043}  &
\showcite{LHCb-PAPER-2011-042}  &
\showcite{LHCb-PAPER-2011-041} \\
\showcite{LHCb-PAPER-2011-040}  &
{\tt LHCb-PAPER-2011-039}\footnote{LHCb-PAPER-2011-039 does not exist.} &
\showcite{LHCb-PAPER-2011-038}  &
\showcite{LHCb-PAPER-2011-037}  &
\showcite{LHCb-PAPER-2011-036} \\
\showcite{LHCb-PAPER-2011-035}  &
\showcite{LHCb-PAPER-2011-034}  &
\showcite{LHCb-PAPER-2011-033}  &
\showcite{LHCb-PAPER-2011-032}  &
\showcite{LHCb-PAPER-2011-031} \\
\showcite{LHCb-PAPER-2011-030}  &
\showcite{LHCb-PAPER-2011-029}  &
\showcite{LHCb-PAPER-2011-028}  &
\showcite{LHCb-PAPER-2011-027}  &
\showcite{LHCb-PAPER-2011-026} \\
\showcite{LHCb-PAPER-2011-025}  &
\showcite{LHCb-PAPER-2011-024}  &
\showcite{LHCb-PAPER-2011-023}  &
\showcite{LHCb-PAPER-2011-022}  &
\showcite{LHCb-PAPER-2011-021} \\
\showcite{LHCb-PAPER-2011-020}  &
\showcite{LHCb-PAPER-2011-019}  &
\showcite{LHCb-PAPER-2011-018}  &
\showcite{LHCb-PAPER-2011-017}  &
\showcite{LHCb-PAPER-2011-016} \\
\showcite{LHCb-PAPER-2011-015}  &
\showcite{LHCb-PAPER-2011-014}  &
\showcite{LHCb-PAPER-2011-013}  &
\showcite{LHCb-PAPER-2011-012}  &
\showcite{LHCb-PAPER-2011-011} \\
\showcite{LHCb-PAPER-2011-010}  &
\showcite{LHCb-PAPER-2011-009}  &
\showcite{LHCb-PAPER-2011-008}  &
\showcite{LHCb-PAPER-2011-007}  &
\showcite{LHCb-PAPER-2011-006} \\
\showcite{LHCb-PAPER-2011-005}  &
\showcite{LHCb-PAPER-2011-004}  &
\showcite{LHCb-PAPER-2011-003}  &
\showcite{LHCb-PAPER-2011-002}  &
\showcite{LHCb-PAPER-2011-001} \\
\hline
\showcite{LHCb-PAPER-2010-002}  &
\showcite{LHCb-PAPER-2010-001} \\
\hline
%  \end{tabular}
\end{longtable}
\end{center}}

{\tiny\begin{center}
\begin{longtable}{lllll}
\caption{\small
  LHCb-CONFs (which have their identifier as their cite code).
  Most CONF notes have been superseded by a paper and are thus retired.
  This is indicated in the bibtex entry. Do not cite retired CONF notes.
   DNE: Does not exist.
}
\label{tab:LHCb-CONFs}
\endfirsthead
\multicolumn{5}{c}{ -- continued from previous page.}
\endhead
\endfoot
\endlastfoot
\hline
% \showcite{LHCb-CONF-2026-005} & 
% \showcite{LHCb-CONF-2026-004} & 
% \showcite{LHCb-CONF-2026-003} & 
% \showcite{LHCb-CONF-2026-002} & 
\showcite{LHCb-CONF-2026-001} \\ 
\hline
\showcite{LHCb-CONF-2025-003} & 
\showcite{LHCb-CONF-2025-002} & 
\showcite{LHCb-CONF-2025-001} \\ 
\hline
\showcite{LHCb-CONF-2024-005} & 
\showcite{LHCb-CONF-2024-004} & 
\showcite{LHCb-CONF-2024-003} & 
\showcite{LHCb-CONF-2024-002} & 
\showcite{LHCb-CONF-2024-001} \\ 
\hline
\showcite{LHCb-CONF-2023-004} & 
\showcite{LHCb-CONF-2023-003} &
\showcite{LHCb-CONF-2023-002} &
\showcite{LHCb-CONF-2023-001} \\
\hline
\showcite{LHCb-CONF-2022-003} & 
\showcite{LHCb-CONF-2022-001} \\ 
\hline
\showcite{LHCb-CONF-2021-005}  &
\showcite{LHCb-CONF-2021-004}  &
\showcite{LHCb-CONF-2021-003}  &
\showcite{LHCb-CONF-2021-002}  &
\showcite{LHCb-CONF-2021-001} \\
\hline
\showcite{LHCb-CONF-2020-003}  &
\showcite{LHCb-CONF-2020-002}  &
\showcite{LHCb-CONF-2020-001} \\
\hline
\showcite{LHCb-CONF-2019-005}  &
\showcite{LHCb-CONF-2019-004}  &
\showcite{LHCb-CONF-2019-003}  &
\showcite{LHCb-CONF-2019-002}  &
\showcite{LHCb-CONF-2019-001} \\
\hline
\showcite{LHCb-CONF-2018-006} \\
\showcite{LHCb-CONF-2018-005}  &
\showcite{LHCb-CONF-2018-004}  &
\showcite{LHCb-CONF-2018-003}  &
\showcite{LHCb-CONF-2018-002}\footnote{If you cite
the gamma combination, always also cite the latest gamma paper as
\texttt{\textbackslash{}cite\{LHCb-PAPER-2013-020,*LHCb-CONF-2018-002\}}
(unless you cite LHCb-PAPER-2013-020 separately too).}  &
\showcite{LHCb-CONF-2018-001} \\
\hline
\showcite{LHCb-CONF-2017-005}  &
\showcite{LHCb-CONF-2017-004}  &
\showcite{LHCb-CONF-2017-003}  &
\showcite{LHCb-CONF-2017-002}  &
\showcite{LHCb-CONF-2017-001} \\
\hline
\showcite{LHCb-CONF-2016-018}  &
\showcite{LHCb-CONF-2016-016} \\
\showcite{LHCb-CONF-2016-015}  &
\showcite{LHCb-CONF-2016-014}  &
\showcite{LHCb-CONF-2016-013}  &
\showcite{LHCb-CONF-2016-012}  &
\showcite{LHCb-CONF-2016-011} \\
\showcite{LHCb-CONF-2016-010}  &
\showcite{LHCb-CONF-2016-009}  &
\showcite{LHCb-CONF-2016-008}  &
\showcite{LHCb-CONF-2016-007}  &
\showcite{LHCb-CONF-2016-006} \\
\showcite{LHCb-CONF-2016-005}  &
\showcite{LHCb-CONF-2016-004}  &
\showcite{LHCb-CONF-2016-003}  &
\showcite{LHCb-CONF-2016-002}  &
\showcite{LHCb-CONF-2016-001} \\
\hline
\showcite{LHCb-CONF-2015-005}  &
\showcite{LHCb-CONF-2015-004}  &
\showcite{LHCb-CONF-2015-003}  &
\showcite{LHCb-CONF-2015-002}  &
\showcite{LHCb-CONF-2015-001} \\
\hline
\showcite{LHCb-CONF-2014-004}  &
\showcite{LHCb-CONF-2014-003}  &
\showcite{LHCb-CONF-2014-002}  &
\showcite{LHCb-CONF-2014-001} \\
\hline
\showcite{LHCb-CONF-2013-013}  &
\showcite{LHCb-CONF-2013-012}  &
\showcite{LHCb-CONF-2013-011} \\
\showcite{LHCb-CONF-2013-010}  &
\showcite{LHCb-CONF-2013-009}  &
\showcite{LHCb-CONF-2013-008}  &
\showcite{LHCb-CONF-2013-007}  &
\showcite{LHCb-CONF-2013-006} \\
\showcite{LHCb-CONF-2013-005}  &
\showcite{LHCb-CONF-2013-004}  &
\showcite{LHCb-CONF-2013-003}  &
\showcite{LHCb-CONF-2013-002}  &
\showcite{LHCb-CONF-2013-001} \\
\hline
\showcite{LHCb-CONF-2012-034}  &
\showcite{LHCb-CONF-2012-033}  &
\showcite{LHCb-CONF-2012-032}  &
\showcite{LHCb-CONF-2012-031} \\
\showcite{LHCb-CONF-2012-030}  &
\showcite{LHCb-CONF-2012-029}  &
\showcite{LHCb-CONF-2012-028}  &
\showcite{LHCb-CONF-2012-027}  &
\showcite{LHCb-CONF-2012-026} \\
\showcite{LHCb-CONF-2012-025}  &
\showcite{LHCb-CONF-2012-024}  &
\showcite{LHCb-CONF-2012-023}  &
\showcite{LHCb-CONF-2012-022}  &
\showcite{LHCb-CONF-2012-021} \\
\showcite{LHCb-CONF-2012-020}  &
\showcite{LHCb-CONF-2012-019}  &
\showcite{LHCb-CONF-2012-018}  &
\showcite{LHCb-CONF-2012-017}  &
\showcite{LHCb-CONF-2012-016} \\
\showcite{LHCb-CONF-2012-015}  &
\showcite{LHCb-CONF-2012-014}  &
\showcite{LHCb-CONF-2012-013}  &
\showcite{LHCb-CONF-2012-012}  &
\showcite{LHCb-CONF-2012-011} \\
\showcite{LHCb-CONF-2012-010}  &
\showcite{LHCb-CONF-2012-009}  &
\showcite{LHCb-CONF-2012-008}  &
\showcite{LHCb-CONF-2012-007}  &
\showcite{LHCb-CONF-2012-006} \\
\showcite{LHCb-CONF-2012-005}  &
\showcite{LHCb-CONF-2012-004}  &
\showcite{LHCb-CONF-2012-003}  &
\showcite{LHCb-CONF-2012-002}  &
\showcite{LHCb-CONF-2012-001} \\
\hline
\showcite{LHCb-CONF-2011-062}  &
\showcite{LHCb-CONF-2011-061} \\
\showcite{LHCb-CONF-2011-060}  &
\showcite{LHCb-CONF-2011-059}  &
\showcite{LHCb-CONF-2011-058}  &
\showcite{LHCb-CONF-2011-057}  &
\showcite{LHCb-CONF-2011-056} \\
\showcite{LHCb-CONF-2011-055}  &
\showcite{LHCb-CONF-2011-054}  &
\showcite{LHCb-CONF-2011-053}  &
\showcite{LHCb-CONF-2011-052}  &
\showcite{LHCb-CONF-2011-051} \\
\showcite{LHCb-CONF-2011-050}  &
\showcite{LHCb-CONF-2011-049}  &
\showcite{LHCb-CONF-2011-048}  &
\showcite{LHCb-CONF-2011-047}  &
\showcite{LHCb-CONF-2011-046} \\
\showcite{LHCb-CONF-2011-045}  &
\showcite{LHCb-CONF-2011-044}  &
\showcite{LHCb-CONF-2011-043}  &
\showcite{LHCb-CONF-2011-042}  &
\showcite{LHCb-CONF-2011-041} \\
\showcite{LHCb-CONF-2011-040}  &
\showcite{LHCb-CONF-2011-039}  &
\showcite{LHCb-CONF-2011-038}  &
\showcite{LHCb-CONF-2011-037}  &
\showcite{LHCb-CONF-2011-036} \\
\showcite{LHCb-CONF-2011-035}  &
\showcite{LHCb-CONF-2011-034}  &
\showcite{LHCb-CONF-2011-033}  &
\texttt{LHCb-CONF-2011-032} DNE &
\showcite{LHCb-CONF-2011-031} \\
\showcite{LHCb-CONF-2011-030}  &
\showcite{LHCb-CONF-2011-029}  &
\showcite{LHCb-CONF-2011-028}  &
\showcite{LHCb-CONF-2011-027}  &
\showcite{LHCb-CONF-2011-026} \\
\showcite{LHCb-CONF-2011-025}  &
\showcite{LHCb-CONF-2011-024}  &
\showcite{LHCb-CONF-2011-023}  &
\showcite{LHCb-CONF-2011-022}  &
\showcite{LHCb-CONF-2011-021} \\
\showcite{LHCb-CONF-2011-020}  &
\showcite{LHCb-CONF-2011-019}  &
\showcite{LHCb-CONF-2011-018}  &
\showcite{LHCb-CONF-2011-017}  &
\showcite{LHCb-CONF-2011-016} \\
\showcite{LHCb-CONF-2011-015}  &
\showcite{LHCb-CONF-2011-014}  &
\showcite{LHCb-CONF-2011-013}  &
\showcite{LHCb-CONF-2011-012}  &
\showcite{LHCb-CONF-2011-011} \\
\showcite{LHCb-CONF-2011-010}  &
\showcite{LHCb-CONF-2011-009}  &
\showcite{LHCb-CONF-2011-008}  &
\showcite{LHCb-CONF-2011-007}  &
\showcite{LHCb-CONF-2011-006} \\
\showcite{LHCb-CONF-2011-005}  &
\showcite{LHCb-CONF-2011-004}  &
\showcite{LHCb-CONF-2011-003}  &
\showcite{LHCb-CONF-2011-002}  &
\showcite{LHCb-CONF-2011-001} \\
\hline
\showcite{LHCb-CONF-2010-014}  &
\showcite{LHCb-CONF-2010-013}  &
\showcite{LHCb-CONF-2010-012}  &
\showcite{LHCb-CONF-2010-011} \\
\showcite{LHCb-CONF-2010-010}  &
\showcite{LHCb-CONF-2010-009}  &
\showcite{LHCb-CONF-2010-008} \\
\multicolumn{5}{c}{Earlier documents in {\tt LHCb-CONF} series are actually proceedings.} \\
\hline
%  \end{tabular}
\end{longtable}
\end{center}}

\section{Standard symbols}

As explained in Sec.~\ref{sec:typography} this appendix contains standard
typesetting of symbols, particle names, units etc.\ in \lhcb
documents.

In the file \texttt{lhcb-symbols-def.tex}, which is included, a
large number of symbols is defined. While they can lead to quicker
typing, the main reason is to ensure a uniform notation within a
document and between different \lhcb documents. If a symbol
like \texttt{\textbackslash CP} to typeset \CP violation is available
for a unit, particle name, process or whatever, it should be used.  If
you do not agree with the notation you should ask to get the
definition in \texttt{lhcb-symbols-def.tex} changed rather than just
ignoring it.

All the main particles have been given symbols. The \B mesons are thus
named \Bp, \Bd, \Bs, and \Bc. There is no need to go into math mode to
use particle names, thus saving the typing of many \$ signs. By
default particle names are typeset in italic type to agree with the
PDG preference. To get roman particle
names you can just change
\texttt{\textbackslash setboolean\{uprightparticles\}\{false\}}
to \texttt{true} at the top of this template.

There is a large number of units typeset that ensures the correct use
of fonts, capitals and spacing. As an example we have
$\mBs=5366.3\pm0.6\mevcc$. Note that \mum is typeset with an upright
$\upmu$, even if the particle names have slanted Greek letters.

A set of useful symbols are defined for working groups. More of these
symbols can be included later. As an example in the Rare Decay group
we have several different analyses looking for a measurement of
\Cpeff7 and \Opep7.

\input{LHCbInternal/lhcb-symbols-list}
